# Supplementary material for: UOD: Unseen Object Detection in 3D Point Cloud
Source: arXiv:2401.03846 source file (2025-05-27)

1-(a)

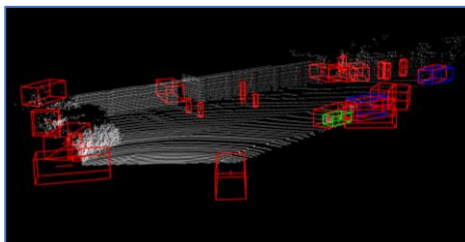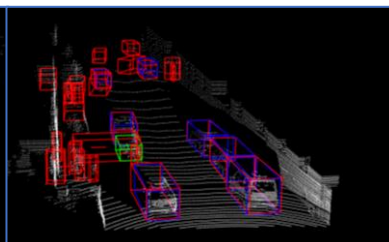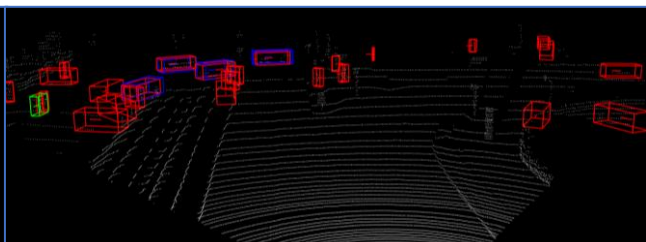

1-(b)

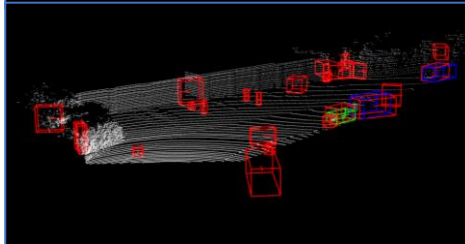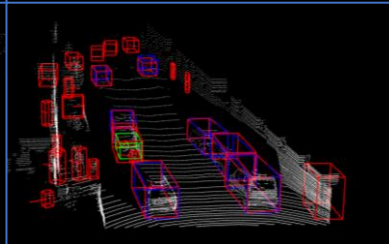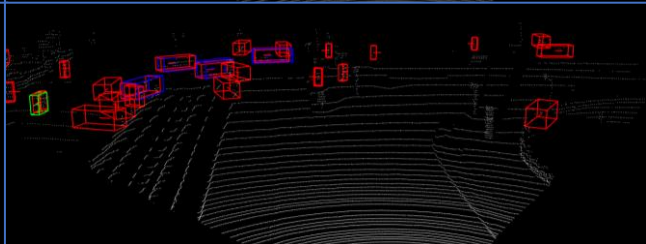

2-(a)

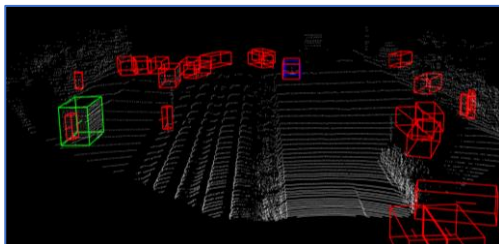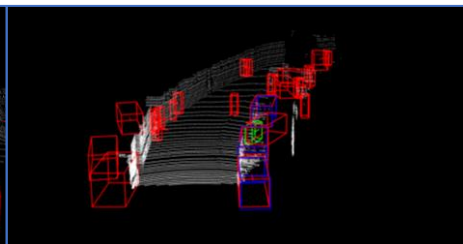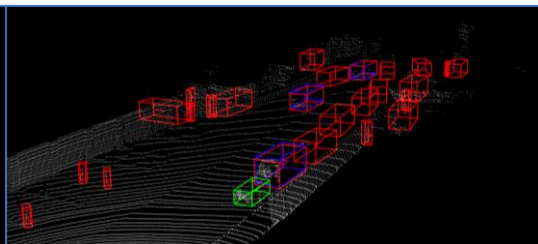

2-(b)

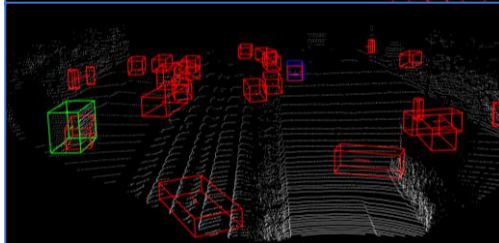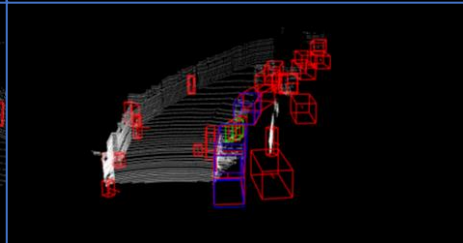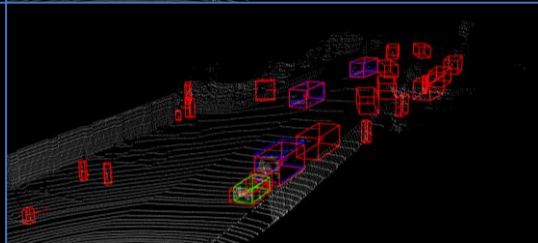

1-(a)

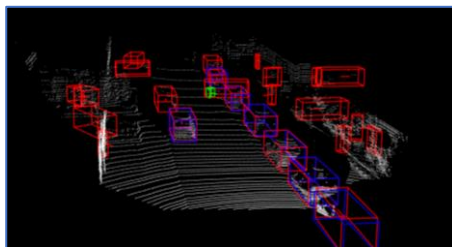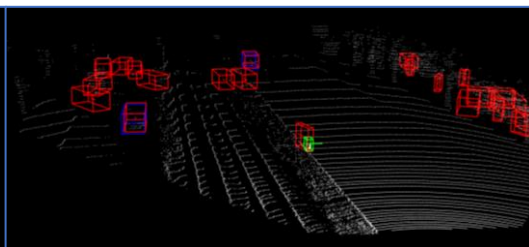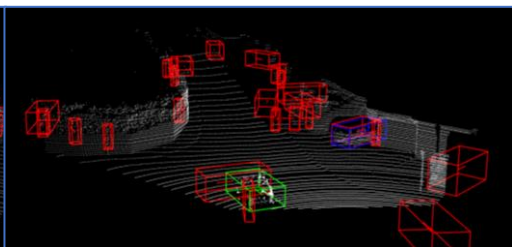

1-(b)

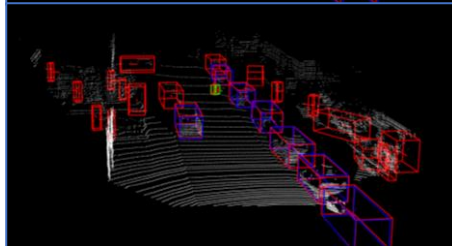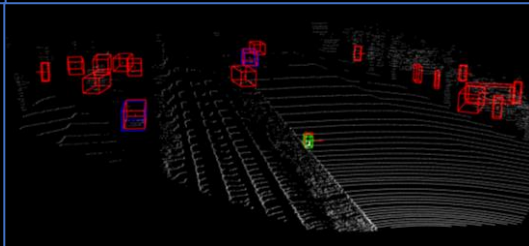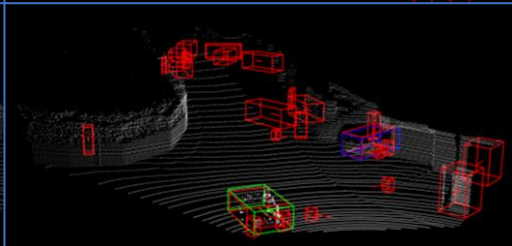

2-(a)

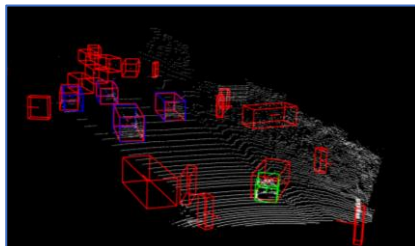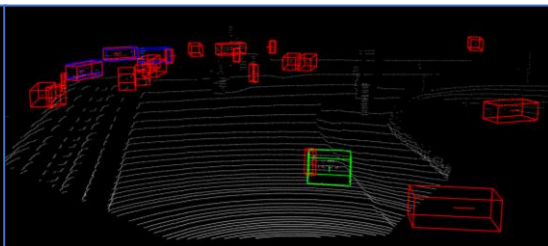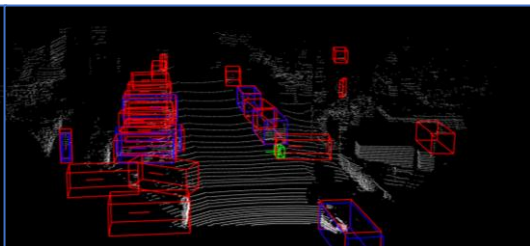

2-(b)

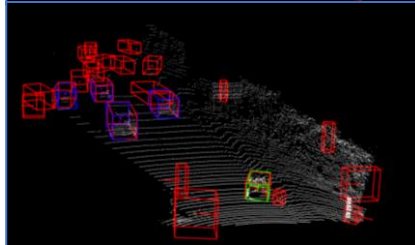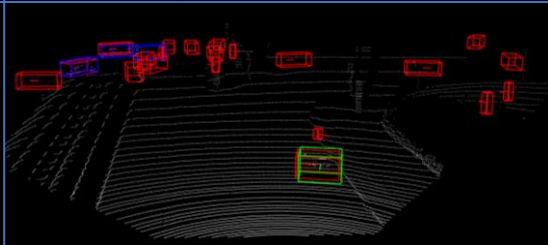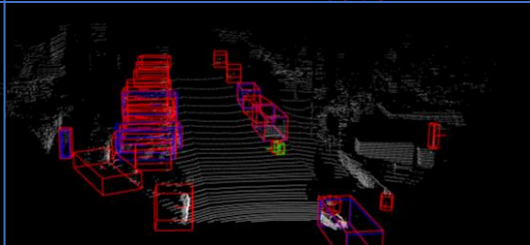

Supplement: Supplementary file 1 [file supp_misc_visual.pdf]
