# Supplementary material for: UOD: Unseen Object Detection in 3D Point Cloud
Source: arXiv:2401.03846 source file (2025-05-27)
Supplement: Supplementary file 3 [file UFO_NUSC_SECOND_table.tex]

% Please add the following required packages to your document preamble:
% \usepackage{multirow}
\begin{table}[t!]
%\captionsetup{font=scriptsize}

\caption{Quantitative result of our method (SECOND) on Nuscenes OOD benchmark.}
\centering
\tiny
\label{NUSC_SECOND}
\begin{tabular}{|c|c|ccc|ccc|}
\hline
\multirow{2}{*}{Nuscenes OOD class}       & Method        & \multicolumn{3}{c|}{Recall @IOU}                                                           & \multicolumn{3}{c|}{OOD detection}                                                         \\ \cline{2-8} 
                                          & SECOND        & \multicolumn{1}{c|}{0.10}           & \multicolumn{1}{c|}{0.25}           & 0.40           & \multicolumn{1}{c|}{AUC$\uparrow$}            & \multicolumn{1}{c|}{AP$\uparrow$}             & FPR$\downarrow$            \\ \hline
\multirow{2}{*}{Debris}                   & Base          & \multicolumn{1}{c|}{28.63}          & \multicolumn{1}{c|}{11.37}          & 3.14           & \multicolumn{1}{c|}{86.95}          & \multicolumn{1}{c|}{86.20}          & 65.69          \\
                                          & \textbf{Ours} & \multicolumn{1}{c|}{\textbf{43.61}} & \multicolumn{1}{c|}{\textbf{31.83}} & \textbf{14.54} & \multicolumn{1}{c|}{\textbf{95.41}} & \multicolumn{1}{c|}{\textbf{96.05}} & \textbf{28.29} \\ \hline
\multirow{2}{*}{Pushable Pullable Object} & Base          & \multicolumn{1}{c|}{21.51}          & \multicolumn{1}{c|}{16.28}          & 7.17           & \multicolumn{1}{c|}{91.41}          & \multicolumn{1}{c|}{92.86}          & 55.23          \\
                                          & \textbf{Ours} & \multicolumn{1}{c|}{\textbf{26.59}} & \multicolumn{1}{c|}{\textbf{22.35}} & \textbf{12.91} & \multicolumn{1}{c|}{\textbf{95.04}} & \multicolumn{1}{c|}{\textbf{94.98}} & \textbf{31.98} \\ \hline
\multirow{2}{*}{Traffic Barrier}          & Base          & \multicolumn{1}{c|}{23.03}          & \multicolumn{1}{c|}{1.62}           & 0.40           & \multicolumn{1}{c|}{88.29}          & \multicolumn{1}{c|}{86.39}          & 59.39          \\
                                          & \textbf{Ours} & \multicolumn{1}{c|}{\textbf{36.49}} & \multicolumn{1}{c|}{\textbf{22.78}} & \textbf{14.31} & \multicolumn{1}{c|}{\textbf{96.13}} & \multicolumn{1}{c|}{\textbf{95.82}} & \textbf{21.77} \\ \hline
\multirow{2}{*}{Traffic Cone}             & Base          & \multicolumn{1}{c|}{29.73}          & \multicolumn{1}{c|}{20.66}          & 7.92           & \multicolumn{1}{c|}{89.42}          & \multicolumn{1}{c|}{90.77}          & 63.51          \\
                                          & \textbf{Ours} & \multicolumn{1}{c|}{\textbf{36.80}} & \multicolumn{1}{c|}{\textbf{26.98}} & \textbf{11.37} & \multicolumn{1}{c|}{\textbf{94.79}} & \multicolumn{1}{c|}{\textbf{94.95}} & \textbf{38.54} \\ \hline
\multirow{2}{*}{Animal}                   & Base          & \multicolumn{1}{c|}{16.83}          & \multicolumn{1}{c|}{2.10}           & 0.00           & \multicolumn{1}{c|}{90.73}          & \multicolumn{1}{c|}{91.64}          & 61.38          \\
                                          & \textbf{Ours} & \multicolumn{1}{c|}{\textbf{38.00}} & \multicolumn{1}{c|}{\textbf{17.08}} & \textbf{4.03}  & \multicolumn{1}{c|}{\textbf{95.93}} & \multicolumn{1}{c|}{\textbf{95.55}} & \textbf{26.30} \\ \hline
\end{tabular}
\end{table}
