# Supplementary material for: UOD: Unseen Object Detection in 3D Point Cloud
Source: arXiv:2401.03846 source file (2025-05-27)
Supplement: Supplementary file 4 [file UFO_detection_BEV_table.tex]

% cifar 10 (q=0.75) / 10 LT (q=0.8) 는 one step
% cifar 100 (q=0.85) / 100 LT (q=0.9) 는 no step

\begin{table}[h!]
%\captionsetup{font=scriptsize}

\caption{Detection BEV (Bird-Eye View) result of our method on the KITTI dataset.}
\centering
\scriptsize
\label{Supp_table_detection_BEV}

\begin{tabular}{|cc|ccc|ccc|lll|}
\hline
\multicolumn{2}{|c|}{\multirow{2}{*}{METHOD}}                       & \multicolumn{3}{c|}{Car BEV AP (R40)}                                        & \multicolumn{3}{c|}{Pedestrian BEV AP (R40)}                                        & \multicolumn{3}{l|}{Cyclist BEV AP (R40)}                                             \\ \cline{3-11} 
\multicolumn{2}{|c|}{}                                              & \multicolumn{1}{c|}{Easy}      & \multicolumn{1}{c|}{Mod}       & Hard      & \multicolumn{1}{c|}{Easy}      & \multicolumn{1}{c|}{Mod}       & Hard      & \multicolumn{1}{c|}{Easy} & \multicolumn{1}{c|}{Mod} & \multicolumn{1}{c|}{Hard} \\ \hline
\multicolumn{1}{|c|}{\multirow{2}{*}{SECOND}}       & Base          & \multicolumn{1}{c|}{}          & \multicolumn{1}{c|}{}          &           & \multicolumn{1}{c|}{}          & \multicolumn{1}{c|}{}          &           & \multicolumn{1}{l|}{}     & \multicolumn{1}{l|}{}    &                           \\
\multicolumn{1}{|c|}{}                              & \textbf{Ours} & \multicolumn{1}{c|}{\textbf{}} & \multicolumn{1}{c|}{\textbf{}} & \textbf{} & \multicolumn{1}{c|}{\textbf{}} & \multicolumn{1}{c|}{\textbf{}} & \textbf{} & \multicolumn{1}{l|}{}     & \multicolumn{1}{l|}{}    &                           \\ \hline
\multicolumn{1}{|c|}{\multirow{2}{*}{PointPillars}} & Base          & \multicolumn{1}{c|}{}          & \multicolumn{1}{c|}{}          &           & \multicolumn{1}{c|}{}          & \multicolumn{1}{c|}{}          &           & \multicolumn{1}{l|}{}     & \multicolumn{1}{l|}{}    &                           \\
\multicolumn{1}{|c|}{}                              & \textbf{Ours} & \multicolumn{1}{c|}{\textbf{}} & \multicolumn{1}{c|}{\textbf{}} & \textbf{} & \multicolumn{1}{c|}{\textbf{}} & \multicolumn{1}{c|}{\textbf{}} & \textbf{} & \multicolumn{1}{l|}{}     & \multicolumn{1}{l|}{}    &                           \\ \hline
\multicolumn{1}{|c|}{\multirow{2}{*}{PV-RCNN}}      & Base          & \multicolumn{1}{c|}{}          & \multicolumn{1}{c|}{}          &           & \multicolumn{1}{c|}{}          & \multicolumn{1}{c|}{}          &           & \multicolumn{1}{l|}{}     & \multicolumn{1}{l|}{}    &                           \\
\multicolumn{1}{|c|}{}                              & \textbf{Ours} & \multicolumn{1}{c|}{\textbf{}} & \multicolumn{1}{c|}{\textbf{}} & \textbf{} & \multicolumn{1}{c|}{\textbf{}} & \multicolumn{1}{c|}{\textbf{}} & \textbf{} & \multicolumn{1}{l|}{}     & \multicolumn{1}{l|}{}    &                           \\ \hline
\multicolumn{1}{|c|}{\multirow{2}{*}{Part A2}}      & Base          & \multicolumn{1}{c|}{}          & \multicolumn{1}{c|}{}          &           & \multicolumn{1}{c|}{}          & \multicolumn{1}{c|}{}          &           & \multicolumn{1}{l|}{}     & \multicolumn{1}{l|}{}    &                           \\
\multicolumn{1}{|c|}{}                              & \textbf{Ours} & \multicolumn{1}{c|}{\textbf{}} & \multicolumn{1}{c|}{\textbf{}} & \textbf{} & \multicolumn{1}{c|}{\textbf{}} & \multicolumn{1}{c|}{\textbf{}} & \textbf{} & \multicolumn{1}{l|}{}     & \multicolumn{1}{l|}{}    &                           \\ \hline
\end{tabular}

\end{table}
